# Supplementary material for: Synthetic Data for Model Selection
Source: arXiv:2105.00717 source file (2023-07-05)
Supplement: Supplementary file 1 [file fig_appendix_imagenet_w_samples_3.tex]

\begin{figure}[H]
    \definecolor{orange}{RGB}{252, 163, 17}
    
    %\fboxsep=-0.5pt %padding thickness
    \fboxrule=0.001\linewidth %border thickness
    \setlength{\fboxsep}{0pt}

    \footnotesize
    \centering
    \setlength{\tabcolsep}{2pt}
    \begin{tabular}{ c  c  c  c  c  c  c}
    \multicolumn{2}{c}{Highest positive $w$} & \multicolumn{2}{c}{Lowest negative $w$} & \multicolumn{2}{c}{$w=0.0$} & $w$ Distribution \\
    \midrule
    $w=0.055$ & $w=0.049$ & $w=-0.070$ & $w=-0.046$ & $w=0.0$ & $w=0.0$ & \\
    \rotatebox{90}{\hspace{2mm}\tiny{Class 250, DiT (cfg=4) \textcolor{white}{p}}}
    \includegraphics[width=0.133\linewidth]{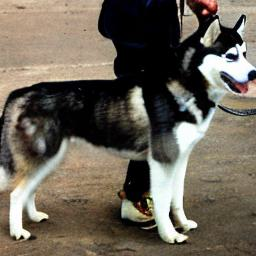} &
    \includegraphics[width=0.133\linewidth]{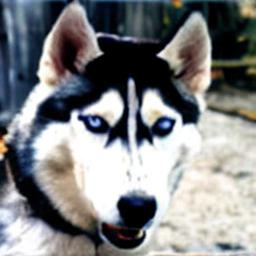} &
    %\frame{
    \includegraphics[width=0.133\linewidth, frame]{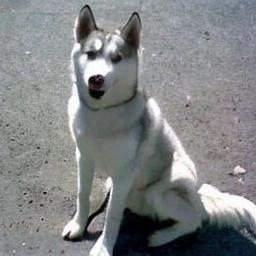} &
    %} &
    %\tcbincludegraphics[]{images/imagenet_w/cfg_4_250/4.jpg} &
    
    \includegraphics[width=0.133\linewidth]{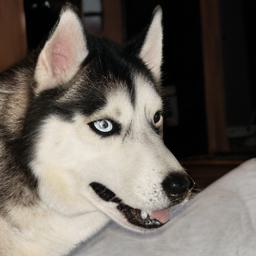} &
    \includegraphics[width=0.133\linewidth]{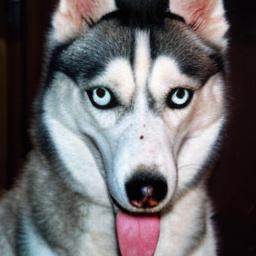} &
    \includegraphics[width=0.133\linewidth]{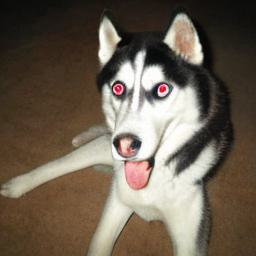} &
    \includegraphics[width=0.133\linewidth]{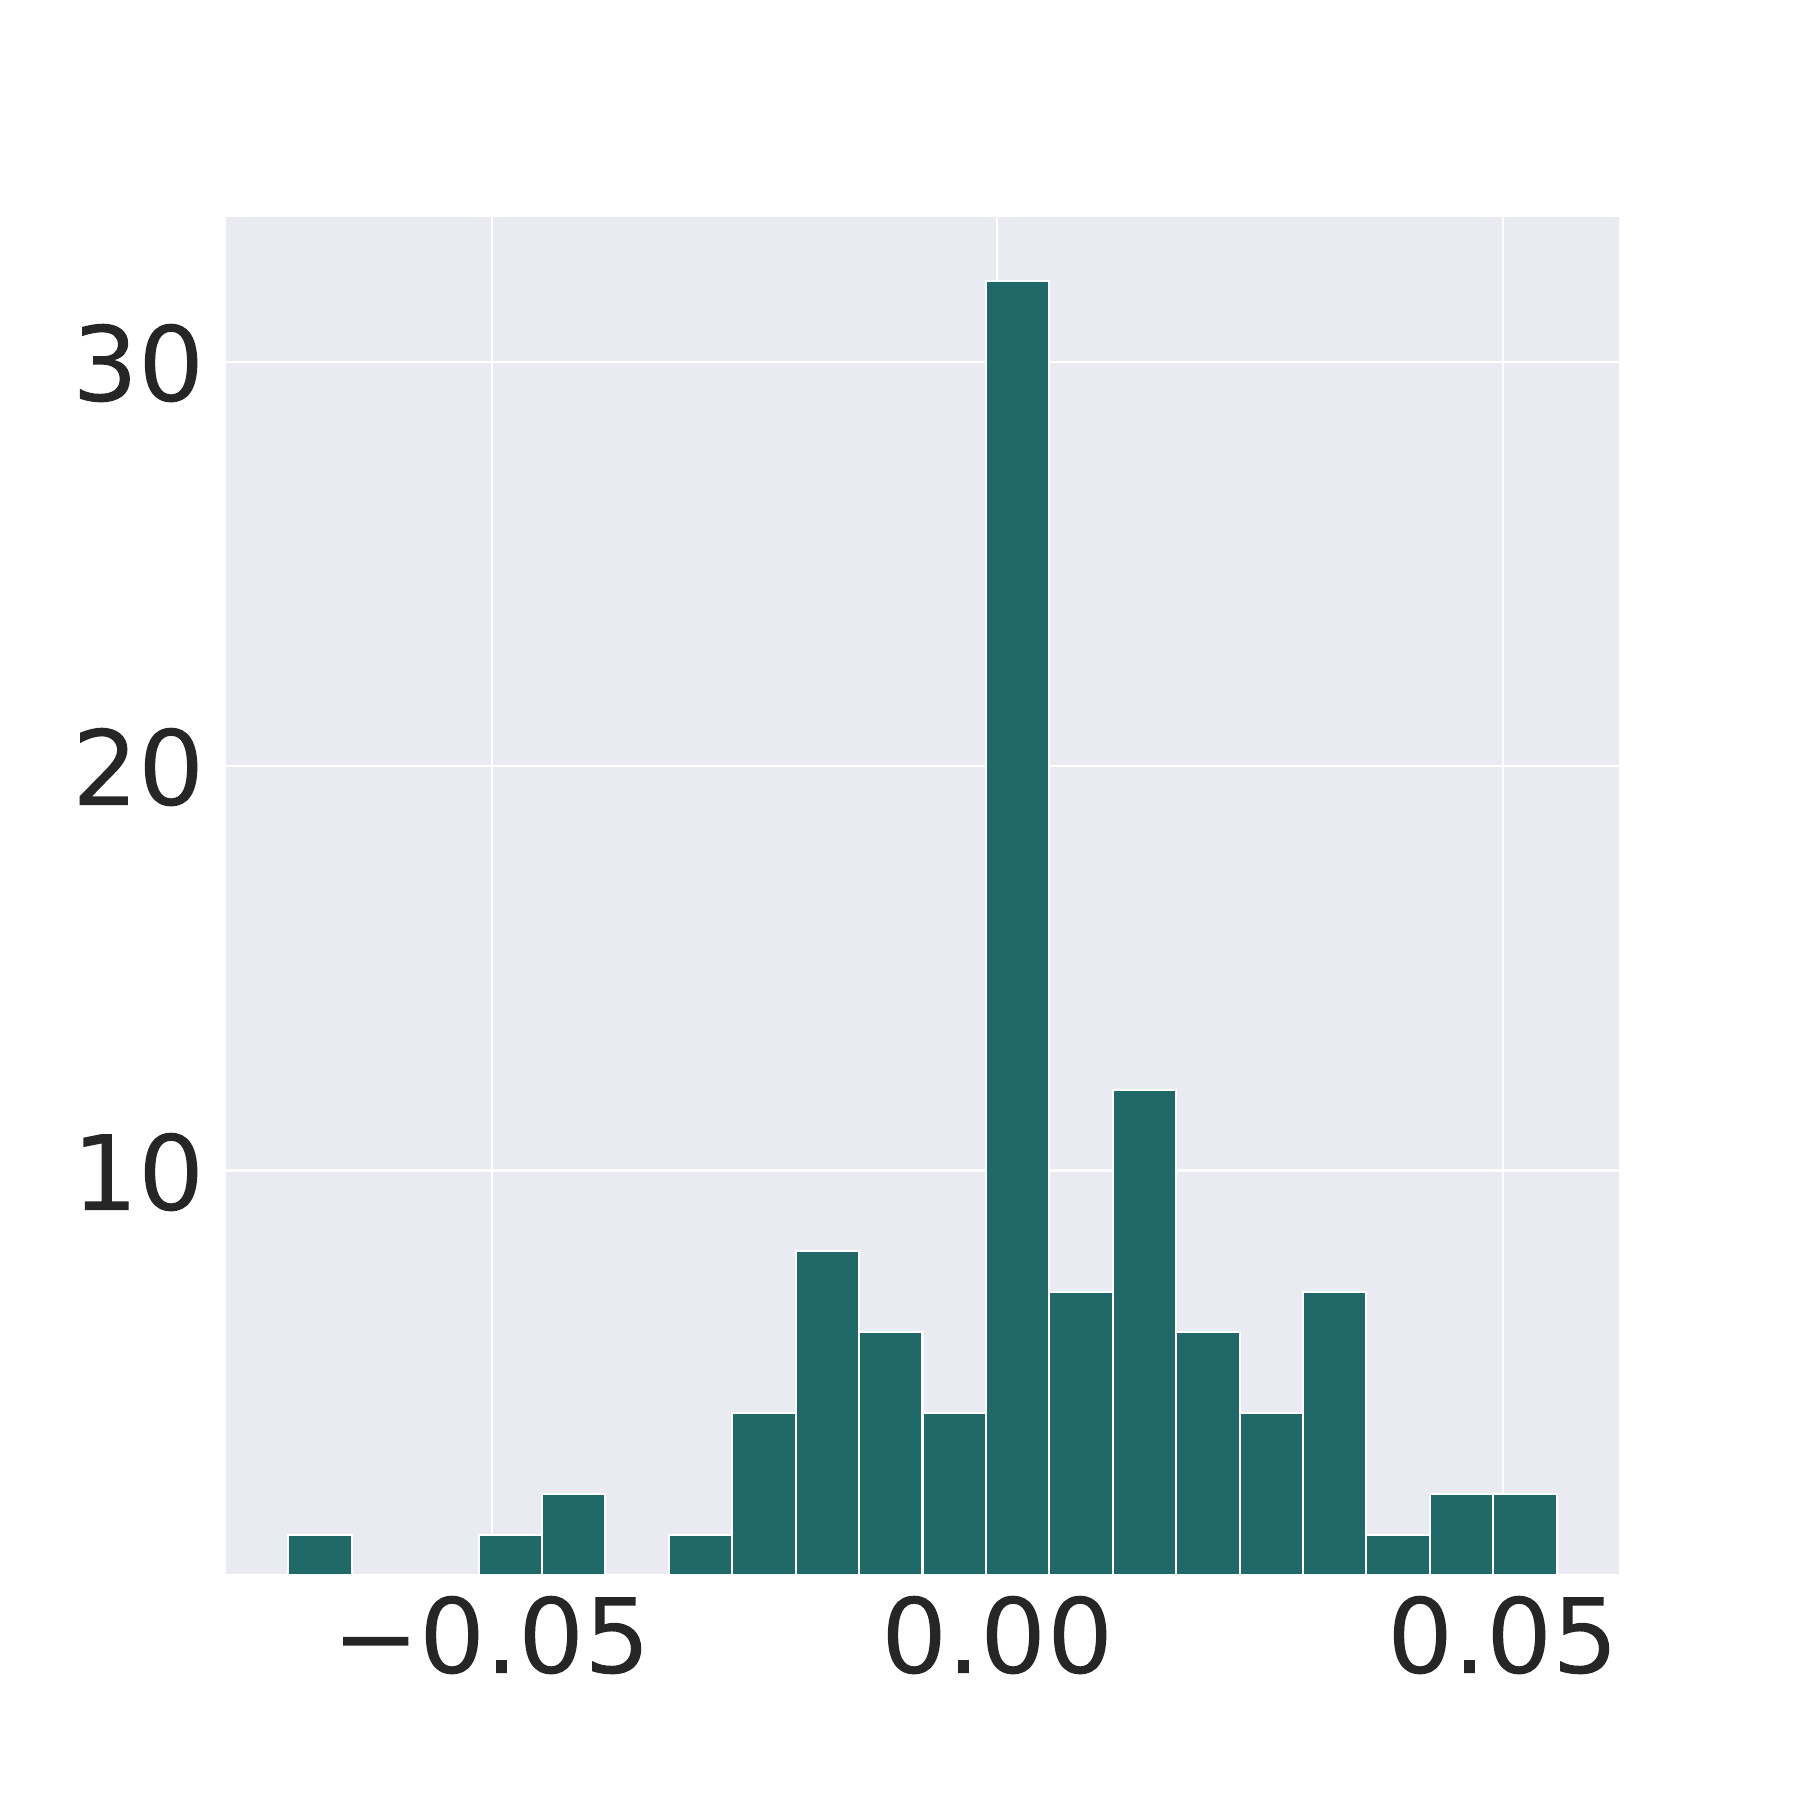} \\
    
    $w=0.063$ & $w=0.060$ & $w=-0.052$ & $w=-0.044$ & $w=0.0$ & $w=0.0$ & \\
    \rotatebox{90}{\hspace{2mm}\tiny{Class 250, DiT (cfg=1) \textcolor{white}{p}}}
    \includegraphics[width=0.133\linewidth]{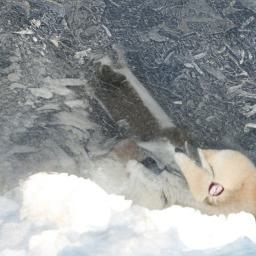} &
    \includegraphics[width=0.133\linewidth]{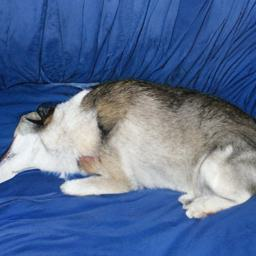} &
    \includegraphics[width=0.133\linewidth]{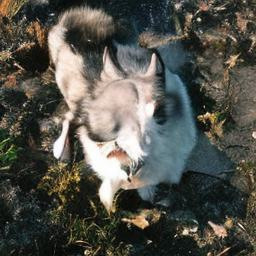} &
    \includegraphics[width=0.133\linewidth]{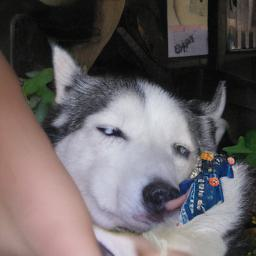} &
    \includegraphics[width=0.133\linewidth]{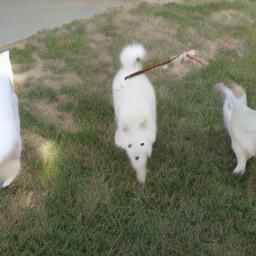} &
    \includegraphics[width=0.133\linewidth]{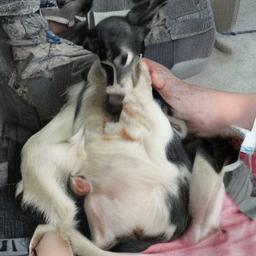} &
    \includegraphics[width=0.133\linewidth]{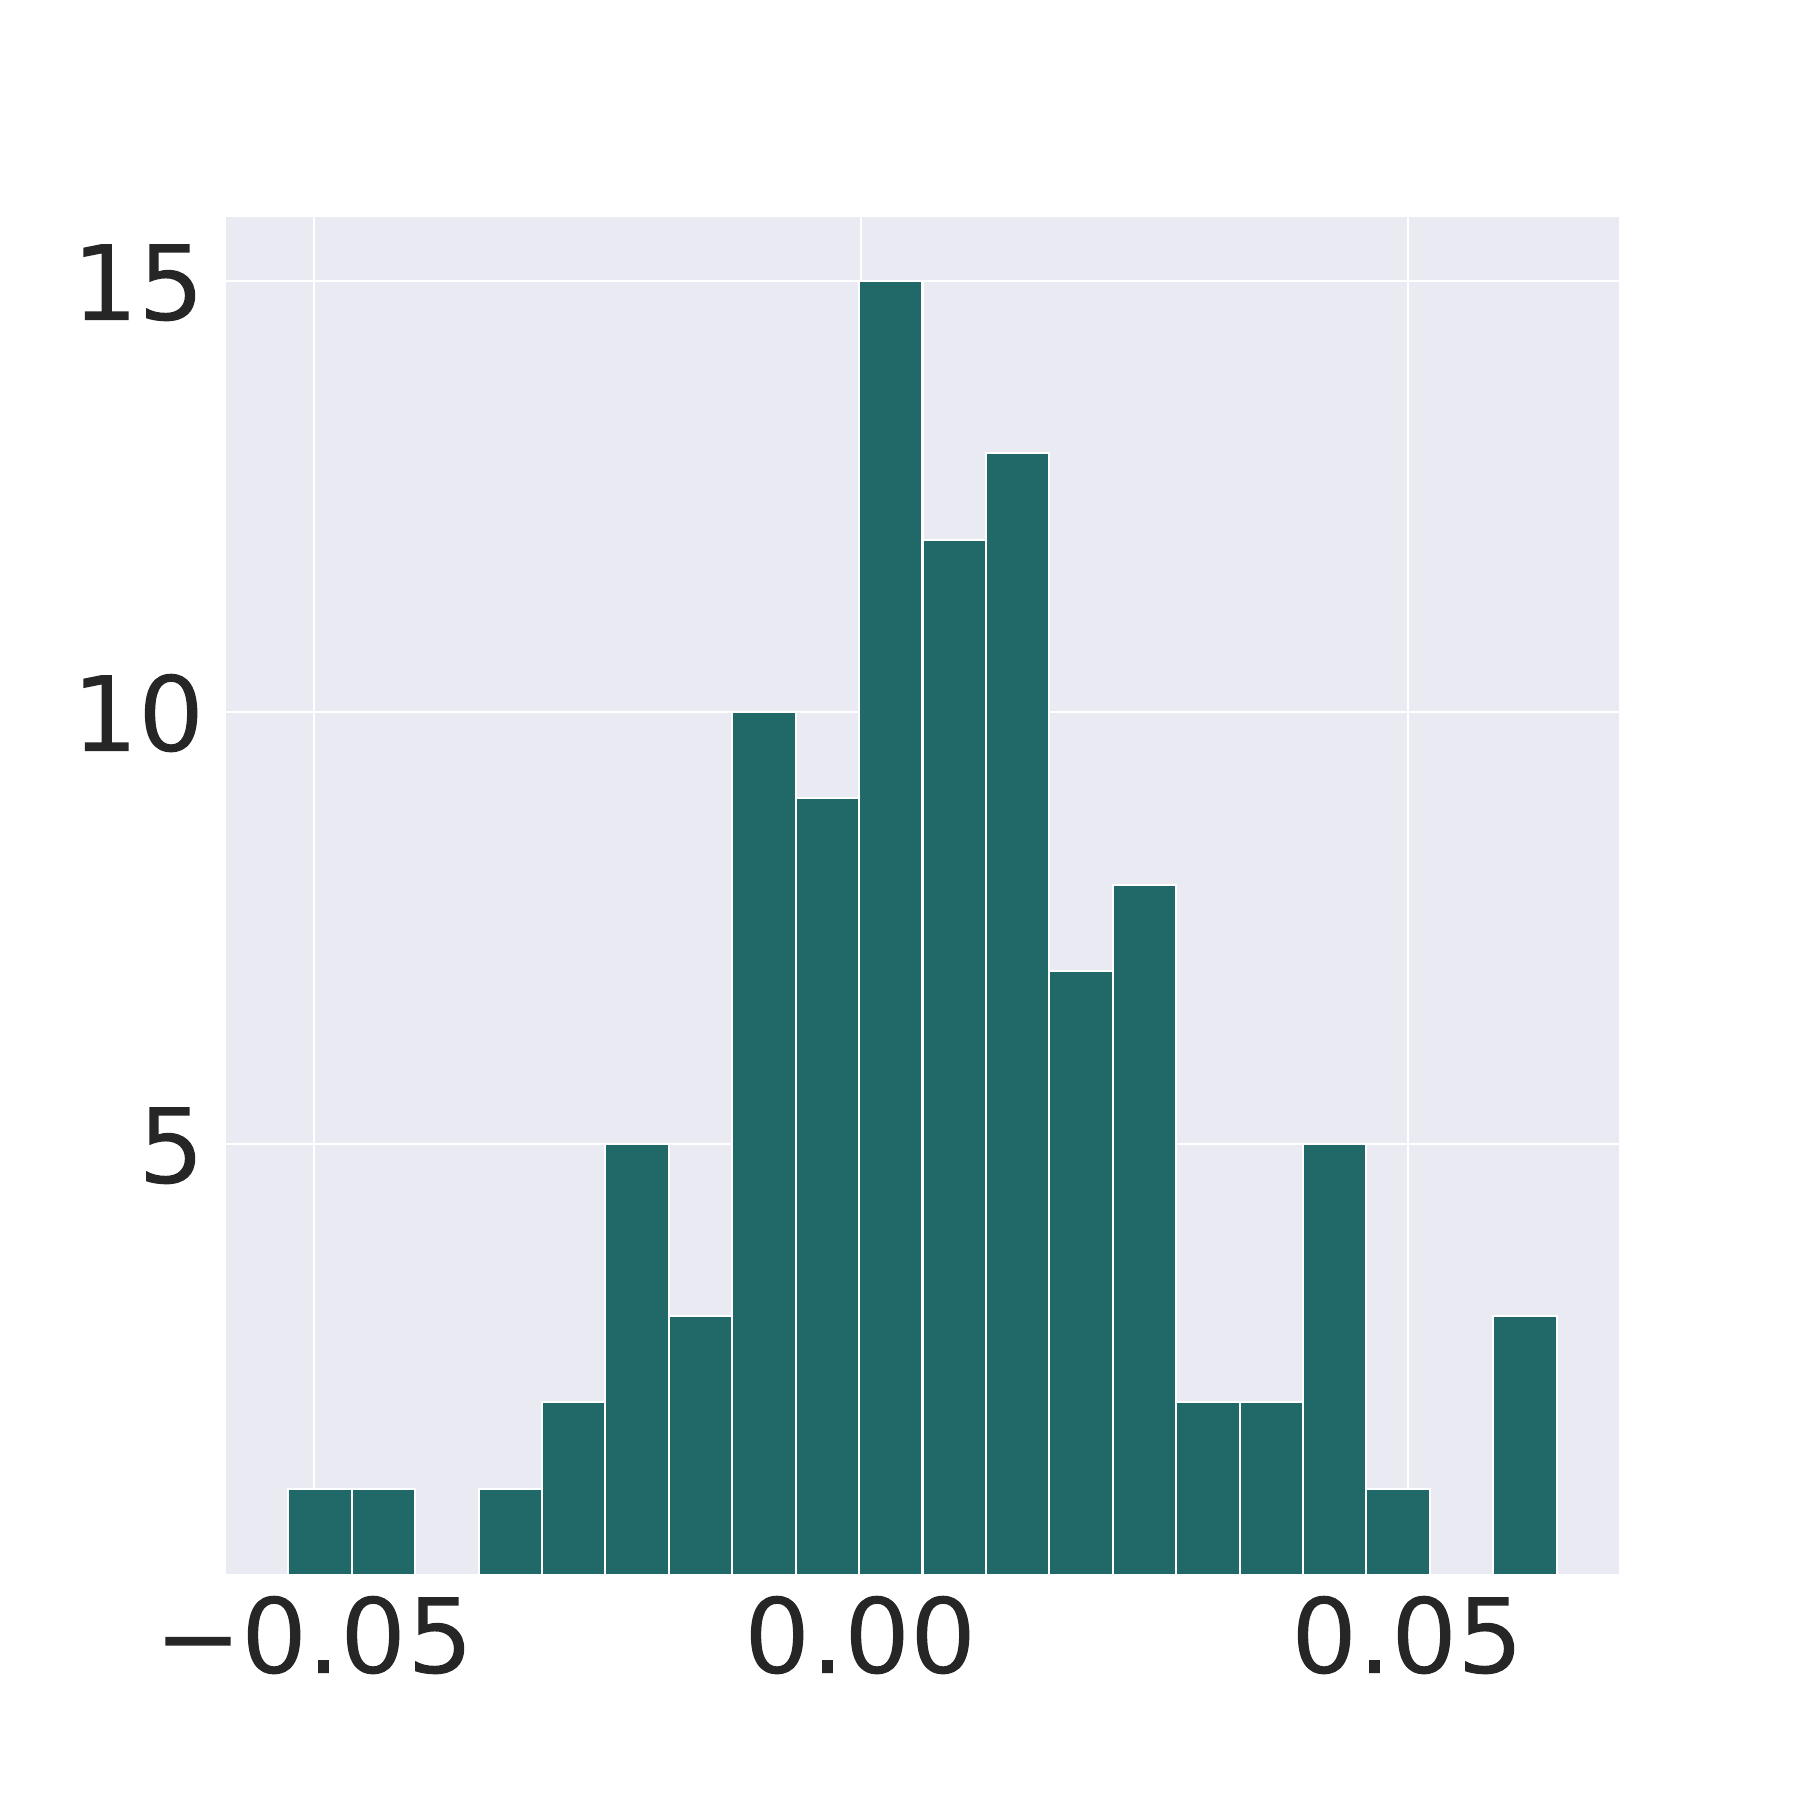} \\
    
    $w=0.066$ & $w=0.043$ & $w=-0.049$ & $w=-0.040$ & $w=0.0$ & $w=0.0$ & \\
    \rotatebox{90}{\hspace{2mm}\tiny{Class 250, BigGAN \textcolor{white}{p}}}
    \includegraphics[width=0.133\linewidth]{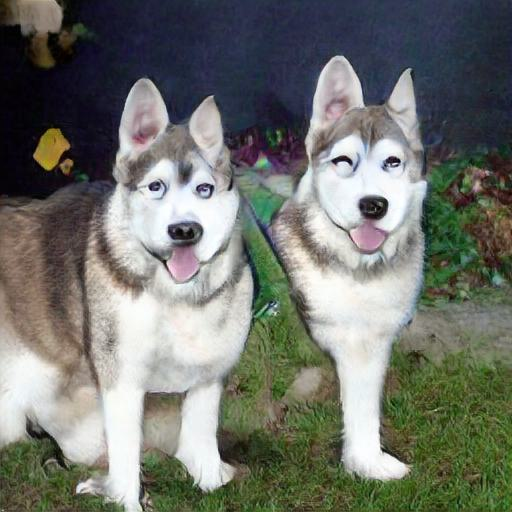} &
    \includegraphics[width=0.133\linewidth]{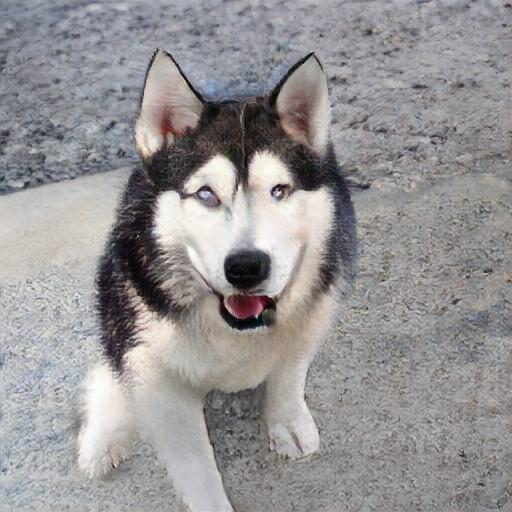} &
    \includegraphics[width=0.133\linewidth]{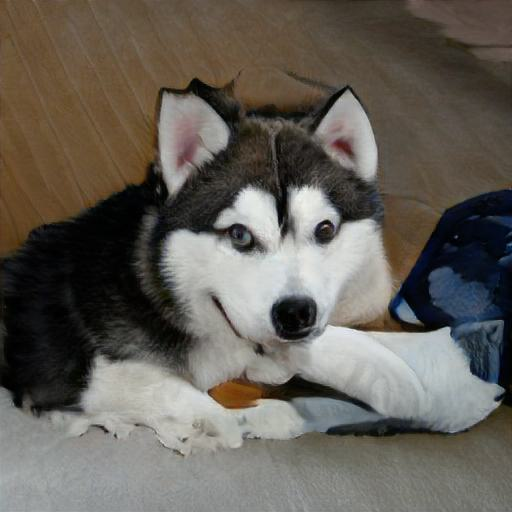} &
    \includegraphics[width=0.133\linewidth]{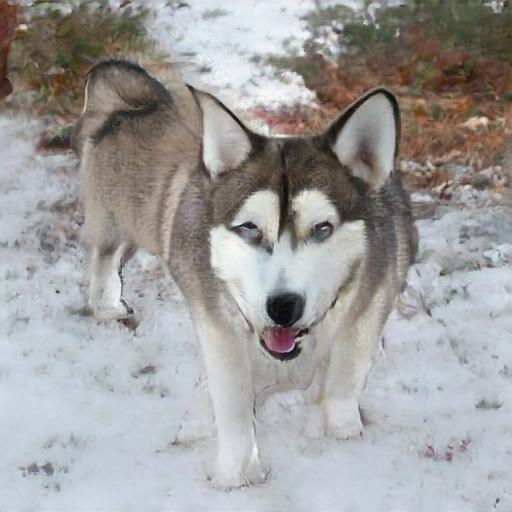} &
    \includegraphics[width=0.133\linewidth]{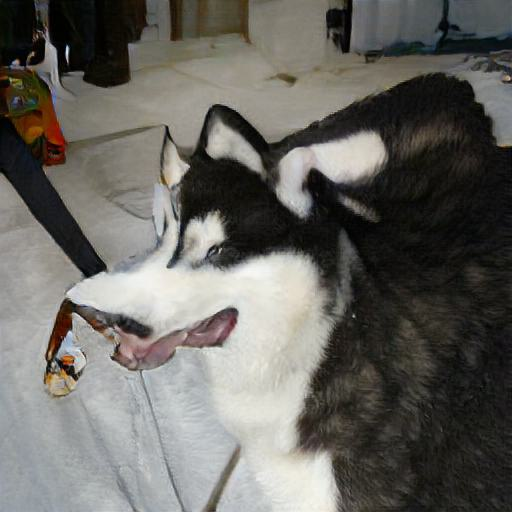} &
    \includegraphics[width=0.133\linewidth]{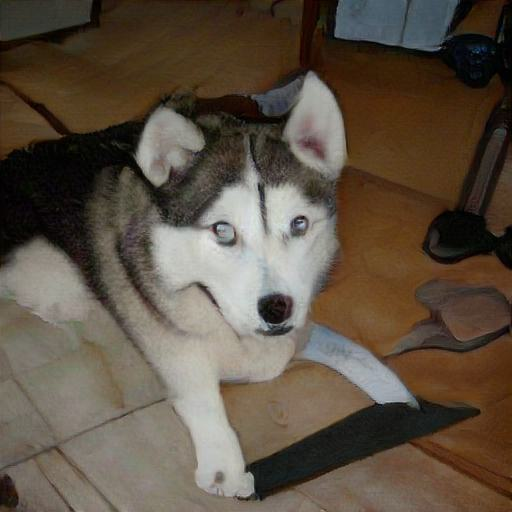} &
    \includegraphics[width=0.133\linewidth]{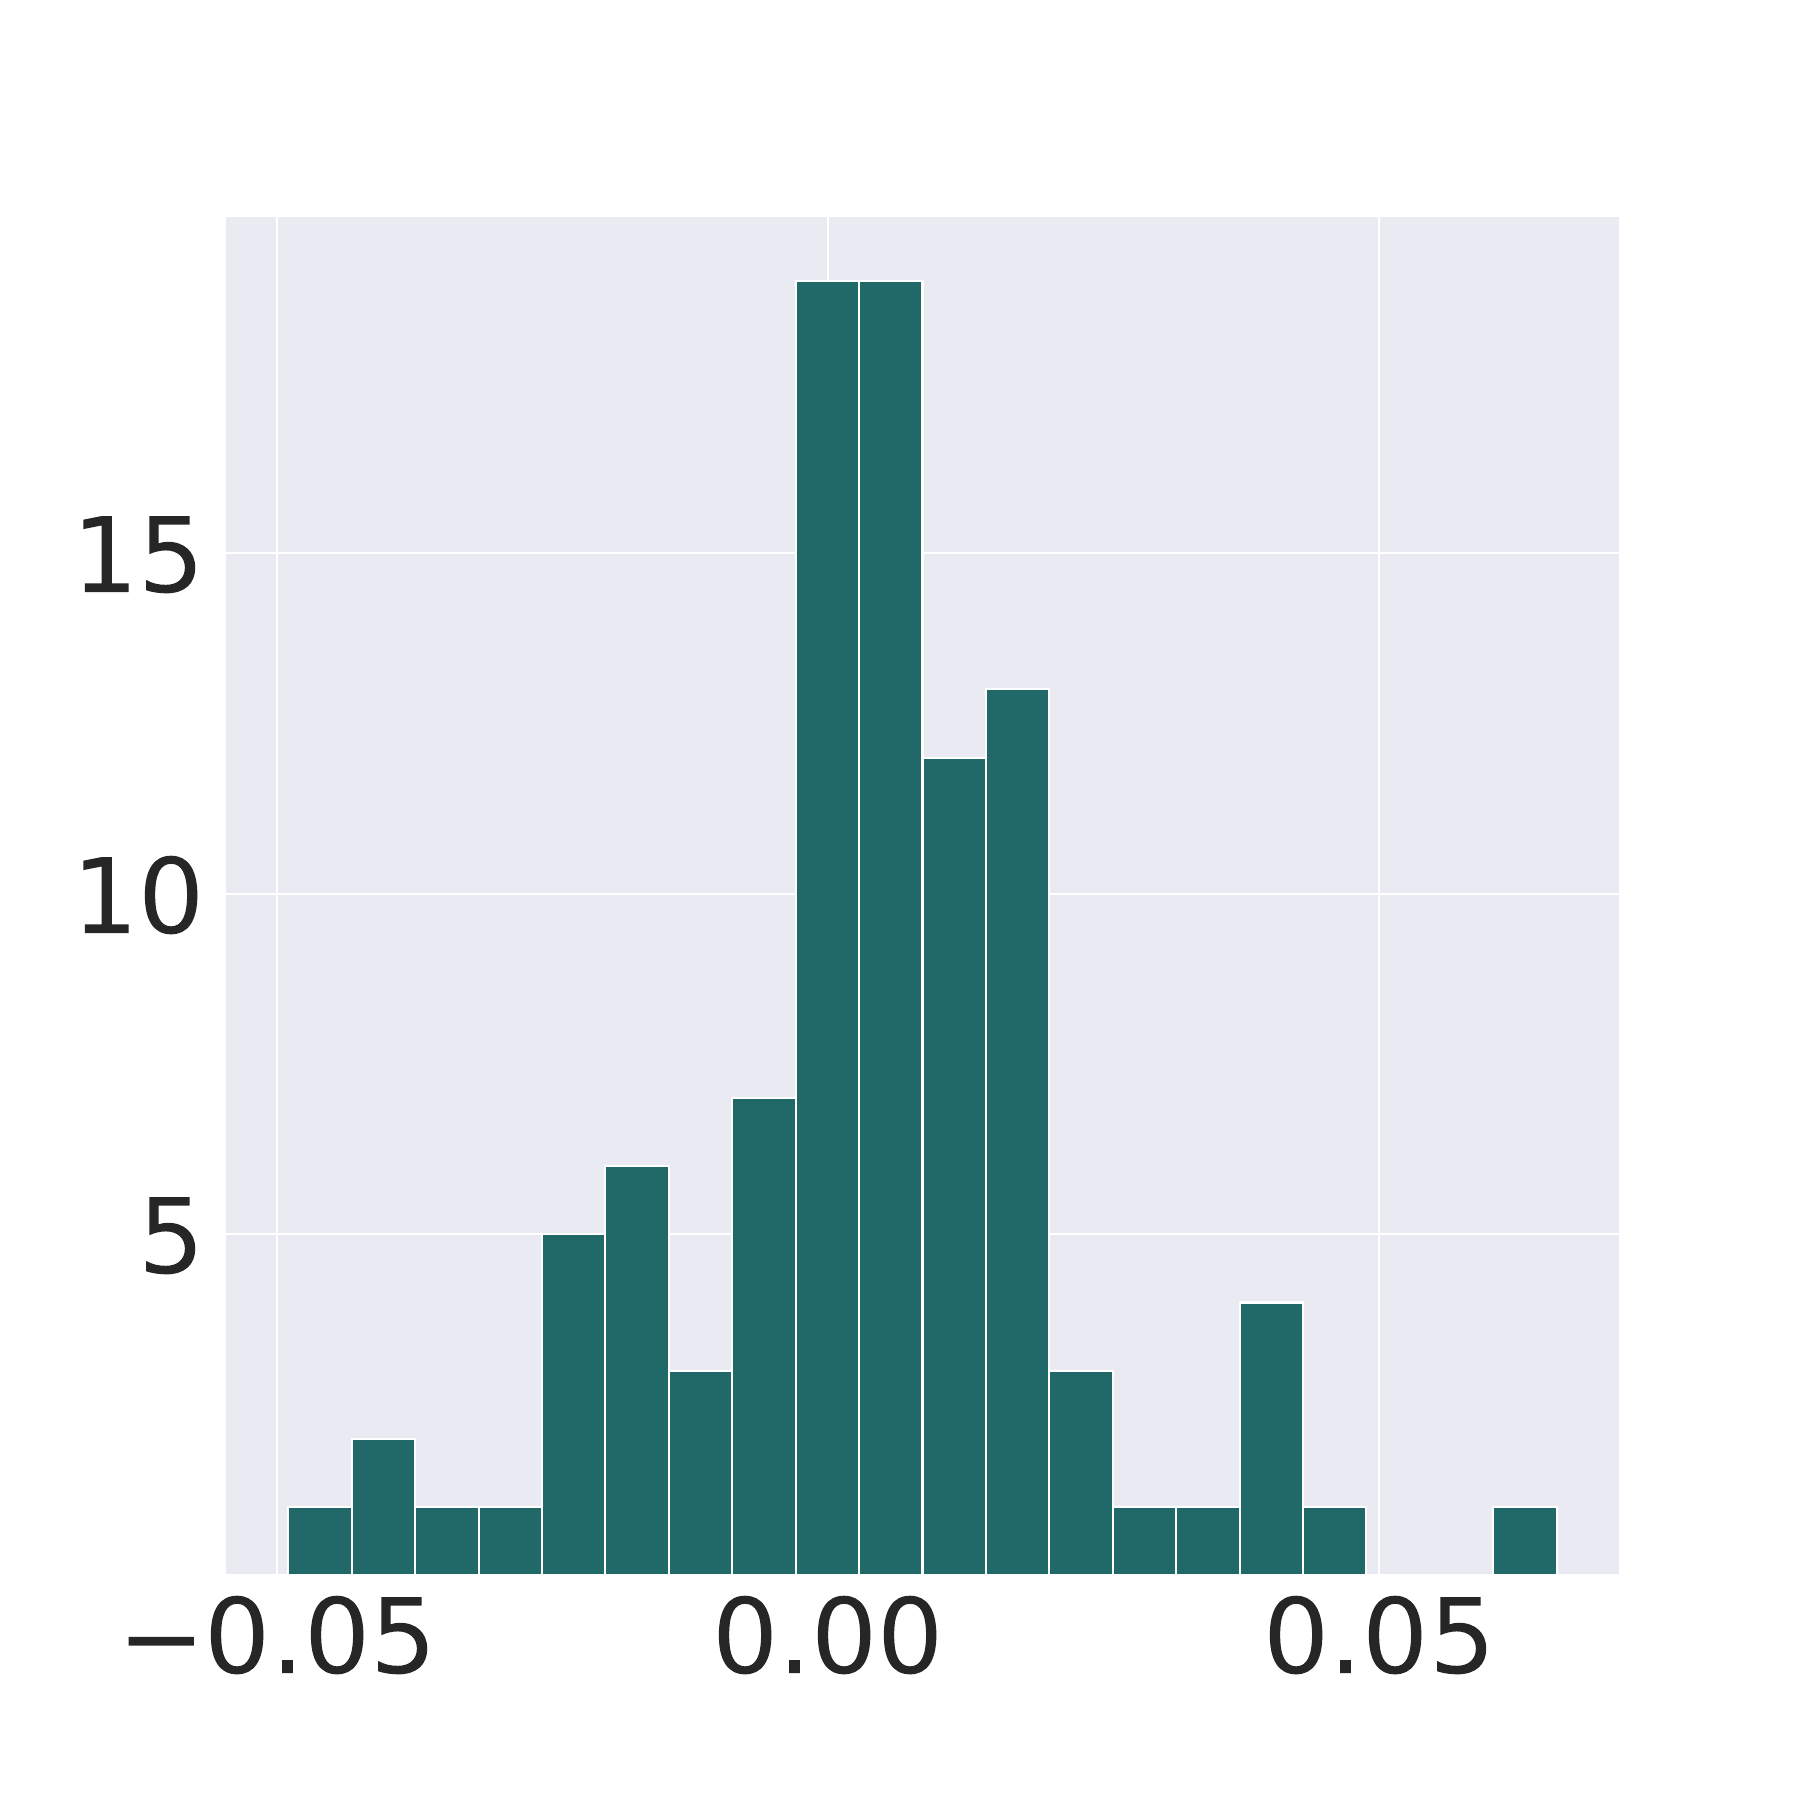} \\
    \end{tabular}
 
\caption{\textbf{Calibrated samples of class ``Siberian husky'' (250):}
First row, columns 3 shown an image that received a low negative number.
It appears that this is a failure of the generative model, as it produced that is more similar to class 248 (Eskimo dog, husky) rather than to the intended class (Siberian Husky). 
Of the models in the calibration set, 21 models classified it as 248 while 29 models classified it as 250, where the highest performing models predicted 248.
Therefore this image is useful for ranking since high performing models tend to agree that this is not a Siberian husky.
First and second row, column 5, received the weight of 0.
The first row received 0 since all classifiers were able to predict the class correctly.
While the image in the second row was ...
First column, second row -- }

% Each row shows images from a different synthetic dataset.
% The first four columns show the images that received the highest positive and lowest negative $w$ coefficient values during calibration.
% Columns five and six show samples that are not useful for ranking and received $w=0$.
% These images are either labeled correctly by all calibration models or labeled ``incorrectly'' by all of them. 
% The last column shows the distribution of $w$ for all 100 images in the class.}
\label{fig:fig_imagenet_w_samples_3}
\end{figure}
